# Supplementary material for: Sound propagation in a uniform superfluid two-dimensional Bose gas
Source: arXiv:1804.04037 ancillary file (2018-04-11)
Supplement: Supplementary file 1 [file supmatv2.pdf]

# Supplemental Material for: Sound propagation in a uniform superfluid two-dimensional Bose gas

J.L. Ville, R. Saint-Jalm, É. Le Cerf, M. Aidelsburger[1,†], S. Nascimbene, J. Dalibard, and J. Beugnon[*]
[1]Laboratoire Kastler Brossel, Collège de France, CNRS, ENS-PSL University, Sorbonne Université, 11 Place Marcelin Berthelot, 75005 Paris, France
(Dated: April 11, 2018)

## PROTOCOL FOR CHARACTERIZING STANDING WAVES

We consider a cloud in a rectangular box of size $L_x \times L_y$. We create an excitation of density at frequency $\omega$ at one end of the rectangle and we choose this excitation to be invariant along the $x$-direction. We decompose this excitation on density modes whose gradient vanishes on the edges of the box and which are invariant along the $x$-direction. We define these spatial modes by $S_j(x,y) = \sqrt{2/(L_xL_y)}\,\cos(k_jy/2)$, where $k_j = 2j\pi/L_y$ and $j \in \mathbb{N}^*$.

In the linear regime, the response of the system is expected to occur at the same frequency $\omega$, and each mode $S_j$ will be excited with an amplitude $B_j(\omega)$ and a phase shift $\varphi_j(\omega)$ with respect to the excitation. Therefore, the density profile at time $t$ will be given by

$$n_{2D}(\omega,t,x,y) = \bar{n}_{2D} + \sum_j B_j(\omega)\sqrt{\frac{2}{L_xL_y}}\cos\left(\frac{k_jy}{2}\right)\cos[\omega t + \varphi_j(\omega)], \quad (1)$$

where $\bar{n}_{2D}$ is the mean density. Our aim is to determine the amplitudes $B_j(\omega)$. However, measuring the full time evolution of $n_{2D}$ for all frequencies would correspond to a large amount of data acquisition. Instead, even without any prior knowledge of $\varphi_j(\omega)$, the amplitudes can be extracted using the following strategy: We measure the density profile at four different times $t_i$, $i \in \{1,2,3,4\}$, and we choose these times so that we explore one oscillation: $\omega t_i = \omega t_1 + (i-1)\pi/2$. We get four density profiles $\rho_i(\omega,y)$, and we compute two quantities $q_1$ and $q_2$:

$$q_1(\omega,y) = \rho_3(\omega,y) - \rho_1(\omega,y) \quad (2)$$
$$= -2\sum_j B_j(\omega)\sqrt{\frac{2}{L_xL_y}}\cos\left(\frac{k_jy}{2}\right)\cos[\omega t_1 + \varphi_j(\omega)], \quad (3)$$

and

$$q_2(\omega,y) = \rho_4(\omega,y) - \rho_2(\omega,y) \quad (4)$$
$$= 2\sum_j B_j(\omega)\sqrt{\frac{2}{L_xL_y}}\cos\left(\frac{k_jy}{2}\right)\sin[\omega t_1 + \varphi_j(\omega)]. \quad (5)$$

We separate the contribution of the different modes by projecting $q_1(\omega,y)$ and $q_2(\omega,y)$ on the eigenmodes of the box:

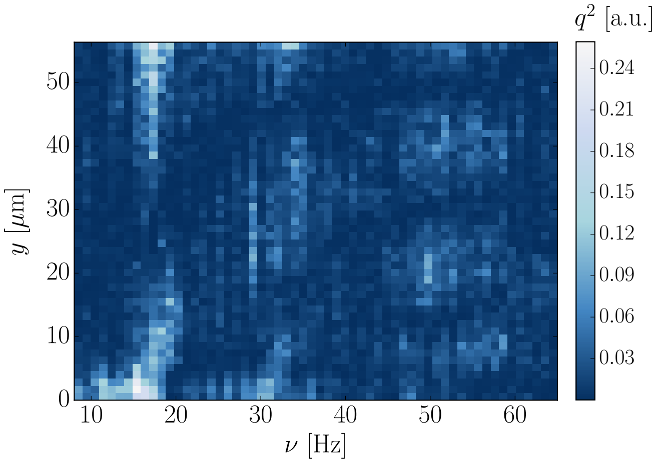


FIG. 1. Integrated spatial profile of the density modulation as a function of the modulation frequency. Each column shows $q^2$ which is the squared amplitude of the density modulation integrated along the $x$ direction, determined from four pictures at different times and averaged over two runs. For this specific experiment, the length of the cloud is $L_y = 57(1)\,\mu$m and the degree of degeneracy is $T/T_c = 0.41(7)$.

$$c_l^{(j)}(\omega) = \sqrt{\frac{2}{L_xL_y}}\int_0^{L_x}\int_0^{L_y} q_l(\omega,y)\cos\left(\frac{k_jy}{2}\right)\mathrm{d}x\,\mathrm{d}y \quad (6)$$
$$= -2B_j(\omega)\cos\left[\omega t_1 + (l-1)\pi/2 + \varphi_j(\omega)\right], \quad (7)$$

for $l = 1$ or 2. The contribution of the $j$-th mode is then given by

$$[B_j(\omega)]^2 = \frac{1}{4}\left(\left[c_1^{(j)}\right]^2 + \left[c_2^{(j)}\right]^2\right). \quad (8)$$

We display in Fig. 4 of the main text a quantity proportional to $B_j^2(\omega)$ for the three first modes.

In addition we also compute the quantity

$$q^2(\omega,y) = q_1^2(\omega,y) + q_2^2(\omega,y), \quad (9)$$

which is displayed in Fig. 1. If the different modes are well separated, the excitation frequency $\omega$ is resonant with at maximum one spatial mode and the sum in Eq. (1) contains only one term. Therefore, we have

$$q^2(\omega,y) \approx 8B_{j_\omega}^2(\omega)/L_y\cos^2(k_{j_\omega}y/2), \quad (10)$$

where $j_\omega$ is the number of the mode that is excited at frequency $\omega$. In this case, $q^2(\omega,y)$ has a simple interpretation:

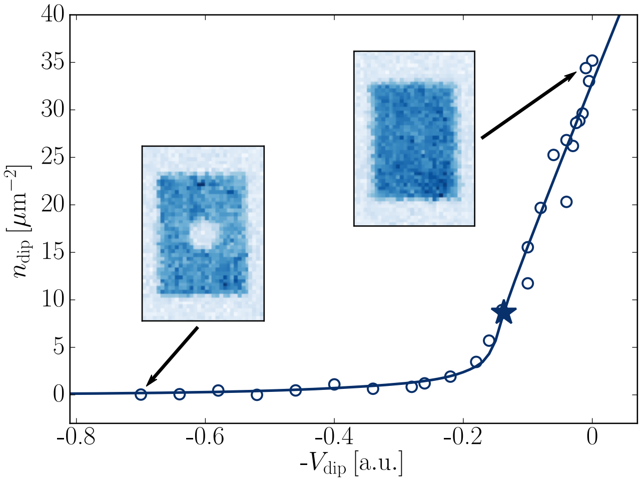


FIG. 2. Surface density in the dip as a function of the applied potential $V_{\text{dip}}$ along with the fit with the equation of state. The two insets are the average of absorption images for two example values of the potential in the dip. The star shows the expected position of the BKT phase transition. The value of the fit to $V_{\text{dip}} = 0$ gives the degree of degeneracy of the cloud. For this cloud we get $T/T_{\text{c}} = 0.21(11)$, where the uncertainty is given by the 95% confidence interval from the fitting procedure. Each data point is the average of three measurements.

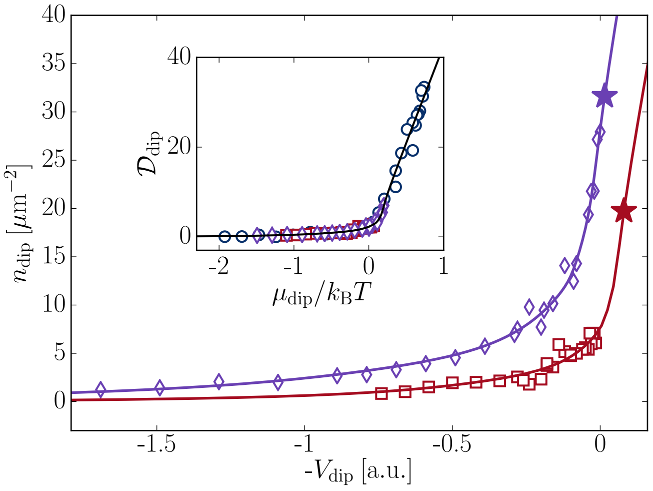


FIG. 3. Two additional examples of the determination of the degree of degeneracy for different parameters (violet diamonds: $T/T_{\text{c}} = 0.95(5)$, red squares: $T/T_{\text{c}} = 1.86(19)$. Each data point is the average of three measurements. The stars correspond to the positions of the BKT phase transition. In the inset we show that all points of Fig. 2 and this figure, when properly rescaled in terms of phase-space density and chemical potential, collapse on the EoS of the 2D Bose gas (black solid line).

It is proportional to the squared amplitude of the mode and it reveals the spatial dependence of the mode with $y$.

## DETERMINATION OF THE DEGREE OF DEGENERACY

The state of a weakly-interacting two-dimensional Bose gas at equilibrium and for a given $\tilde{g}$ can be characterized by a single dimensionless parameter, for instance $T/T_{\text{c}}$ or equivalently its phase-space density $\mathcal{D} = n_{\text{2D}}\lambda_T^2$, where $\lambda_T^2 = 2\pi\hbar^2/(mk_BT)$. Taking advantage of this scale invariance, we use here a method inspired from [1] to determine directly the phase-space density of the cloud without independent measurements of the atomic density and the temperature, and hence without accumulating errors in these two calibrations.

The principle of the measurement is to use an additional potential $V_{\text{dip}}$ in a small region of the cloud (dip zone). Atoms inside this zone are in thermal equilibrium with the rest of the cloud but they experience an effective local chemical potential $\mu_{\text{dip}}$ shifted from the overall chemical potential $\mu$: $\mu_{\text{dip}} = \mu - V_{\text{dip}}$. By measuring the surface density in the dip as a function of $V_{\text{dip}}$ and using the known equation of state (EoS) of the gas, we determine the degree of degeneracy of the cloud.

In more detail, we shine on the cloud confined in the usual box potential an additional disk-shaped repulsive laser beam, as shown in the insets of Fig. 2. The disk-shaped region has to be small enough so that the change of potential in this part does not influence the rest of the gas: We use here a disk of radius 5 µm in a rectangle of 30 µm × 38 µm which corresponds to approximately 7 % of the total area of the box.

We now write the equation of state of the gas with phase-space density $\mathcal{D}$ and in the dip zone with phase-space density $\mathcal{D}_{\text{dip}}$,

$$\mathcal{D} = f\left(\frac{\mu}{k_{\text{B}}T}\right) \quad \text{and} \quad \mathcal{D}_{\text{dip}} = f\left(\frac{\mu_{\text{dip}}}{k_{\text{B}}T}\right), \tag{11}$$

where we have assumed equal temperatures for the two regions and where $\mu_{\text{dip}} = \mu - V_{\text{dip}}$. The function $f$ describes the equation of state of the 2D Bose gas. Introducing the surface densities $n$ and $n_{\text{dip}}$ in the main region and in the dip of the cloud we get

$$n = \frac{1}{\lambda_T^2} f\left(\frac{\mu}{k_{\text{B}}T}\right) \quad \text{and} \quad n_{\text{dip}} = \frac{1}{\lambda_T^2} f\left(\frac{\mu - V_{\text{dip}}}{k_{\text{B}}T}\right). \tag{12}$$

A typical measurement of the surface density $n_{\text{dip}}$ as a function of the applied potential $V_{\text{dip}}$ is shown in Fig. 2. For a large value of the potential $V_{\text{dip}}$ the density tends to zero in the dip (see left inset). In the limit of no additional potential we recover a uniform density distribution (see right inset). Note that the range of measured $n_{\text{dip}}$ being large we use a partial imaging method [2] to adjust the density of cloud probed with our absorption imaging beam. It is indeed crucial that the measured optical depth scales linearly with the atomic density and it is known that it is not the case for optically dense samples [3].

The data points are then fitted with a rescaled EoS:

$$n_{\text{dip}} = p_1 f\left(\frac{p_2 - V}{p_3}\right), \tag{13}$$

where $p_1$, $p_2$ and $p_3$ are three fitting parameters. The phase-space density $\mathcal{D}_{\rm dip}$ then simply reads

$$\mathcal{D}_{\rm dip} = \frac{n_{\rm dip}}{p_1}. \tag{14}$$

The same fitting parameter $p_1$ is used to extract the phase-space density $\mathcal{D} = n/p_1$ of the unperturbed gas. The results of this procedure for different clouds are shown in Fig. 3 along with their determined degree of degeneracy.

## DENSITY CALIBRATION

Atom number calibration is a difficult task in our system because of the important role of dipole-dipole interactions in standard absorption imaging techniques [3] and the complex atomic level structure of the Rb atom. In this work we use the method inspired from Ref. [4]. Starting from a dilute cloud trapped in the optical box potential and in the $|F = 1, m = 0\rangle$ state, we use a $\pi/2$ microwave pulse to create a coherent superposition of this initial state with the $|F = 2, m = 0\rangle$ state. We measure independently the populations $N_1 \approx N/2$ and $N_2 \approx N/2$ in these two states for each experimental run, where $N$ is the total atom number in the region of interest. We extract from typical sets of a hundred measurements the variance of the population difference $\mathrm{Var}(N_2 - N_1)$, which for a pure projection measurement, equals to $N$ and then allows one to determine the atom number.

From this calibration we deduce that the cross-section for our absorption imaging is decreased by a factor 1.8(0.2) with respect to the two-level case with an infinitely narrow line: $\sigma_0 = (7/15) \times 3\lambda^2/(2\pi)$, where $\lambda$ is the resonant wavelength. The factor 7/15 originates from the average of the Clebsch-Gordan coefficients for $\pi-$polarized light resonant with the $|F = 2\rangle$ to $|F = 3\rangle$ $D_2$ transition, as used in our experiment. This projection noise calibration is done with clouds with a typical optical depth of 0.4. The measurements of the cloud's density for determining the Bogoliubov speed of sound were done with a larger optical depth around 1. Using the results from Ref. [3], we then add another correction of 15% to take into account the decrease of the cross-section because of light-induced dipole-dipole interactions for an optical depth of 1 compared to 0.4. In conclusion, we correct our bare measurements of optical depth by $\eta = 2.07(0.23)$. Note that this correction is only used for the scaling of the vertical axis of Fig. 3a of the main text, and that all the measurements reported in the main text are independent of the correction factor thanks to the direct determination of the degree of degeneracy of the cloud described above.

## COMPLEMENTARY RESULTS

The degree of degeneracy of the gas is scanned by varying both the sample's temperature and density. The bare results for the measured $c$, without dividing by $c_{\rm B}$, are shown in Fig. 4a. The temperature of the sample can be extracted from the measurement of the degree of degeneracy of the cloud and of its density, as $\mathcal{D} \propto n_{\rm 2D}/T$. The resulting temperatures are shown by the color of the points in Fig. 4.

The density is varied by a factor 7 and the temperature by a factor 4. Figs. 4b and 4c display the same results as in the main text but showing the temperature for each data point. The collapsing of all the points of Fig. 4 on a single curve in Fig. 4b is expected for the propagation of sound in the hydrodynamic regime in weakly-interacting 2D Bose gases, due to their scale-invariant behavior.

## LANDAU DAMPING

Landau damping mechanism describes the decay of phonons due to interaction with thermal excitations. Landau damping rate $\Gamma$ for two-dimensional systems has been computed in Refs. [5, 6]. The damping of a given sound mode can be characterized by a dimensionless quality factor $Q = \omega/\Gamma$, where $\omega/2\pi$ is the mode frequency. This quality factor is independent of the mode and only depends in 2D on the dimensionless ratio $T/T_{\rm c}$. Its explicit expression, which is plotted in Fig. 3b of the main text is

$$1/Q(\tau) = \frac{\tilde{g}}{16\pi\tau}\times \int_0^\infty dx \left(\frac{2}{\sqrt{1+x^2}} + \frac{1}{1+x^2}\right)^{3/2} (\sqrt{1+x^2}-1)\,\mathrm{Csch}^2[x/(2\tau)], \tag{15}$$

where $\mathrm{Csch} = 1/\sinh$ and

$$\tau = \frac{2\pi}{\tilde{g}\ln(380/\tilde{g})}\frac{T}{T_{\rm c}}. \tag{16}$$

In the regime $T/T_c \gg \tilde{g}/(2\pi)$ relevant in our experiments, the integral can be approximated by its asymptotic expression for $\tau \gg 1$, leading to the simplified expression

$$Q \simeq \frac{2}{\pi}\ln(380/\tilde{g})\frac{T_{\rm c}}{T}.$$

In the opposite regime of very low temperatures $T/T_c \ll \tilde{g}/(2\pi)$, we find the asymptotic behavior

$$Q \simeq \frac{2}{\sqrt{3\pi^3}}\tilde{g}\ln(380/\tilde{g})^2\left(\frac{T_{\rm c}}{T}\right)^2.$$

We remind that for bosonic superfluids in 3D, including liquid $^4$He, the Landau damping rate scales as $T^4$ in the low-temperature regime, i.e. $Q \propto 1/T^4$ [7].

## INFLUENCE OF THE EXCITATION

We checked that our measurements of speed of sound are independent of the details of the excitation protocol. We show

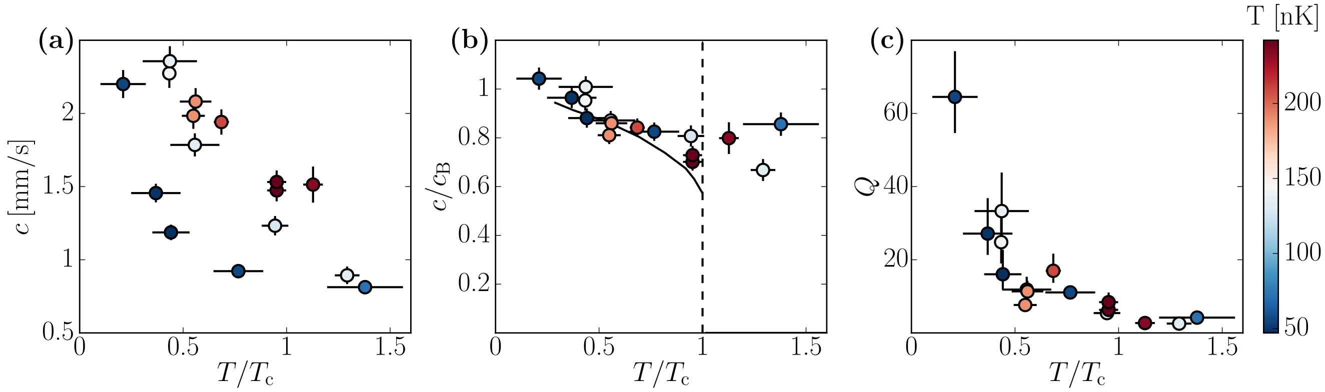


FIG. 4. Speed of sound and damping. (a) Speed of sound (not normalized to Bogoliubov speed of sound). The color code gives the temperature for each point. The variation of $c$ from 0.8 to 2.5 mm/s is mainly due to the change of density of the cloud. (b) Measured speed of sound normalized to the Bogoliubov speed of sound $c_\mathrm{B}$ with the same color code as in (a) (c) Quality factor $Q = \omega/\Gamma$ of the first mode determined for the experimental points with the same color code as in (a).

in Fig. 5a the influence of the amplitude of the excitation dip (where the density is about 2/3 of the total density in the main text) and observe no important variation of the speed of sound even for an almost full depletion in the dip region. We report in Fig. 5b the influence of the size of the excitation region (25% of the box length in the main text) and also observe no strong influence of this parameter. We also studied the damping of the sound waves as a function of the excitation strength (not shown here). For strong excitation ($\approx$ full depletion of the initial cloud) we observed a faster damping of the oscillations, but we checked that decreasing the excitation strength with respect to the configuration studied in the main text does not lead to significant variations of the damping rate.

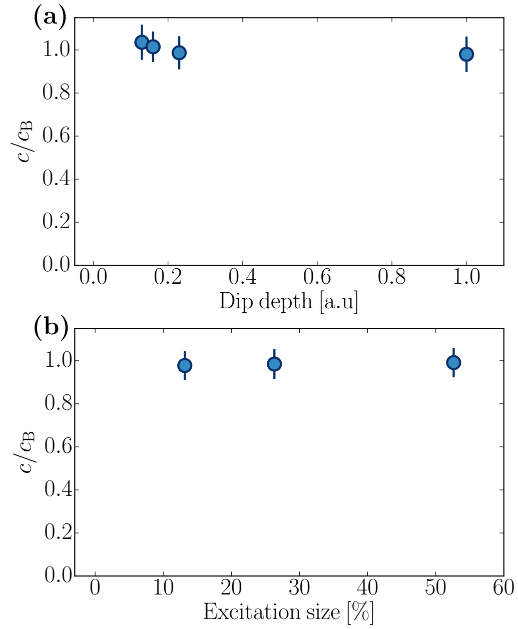


FIG. 5. Normalized speed of sound for a gas in the degenerate regime ($T/T_\mathrm{c} \approx 0.25$) for different excitation protocols. (a) Influence of depth of the excitation dip. The data in the main text were taken for a dip depth of 0.16 a.u.. The value of 1 corresponds to an almost fully depleted dip. (b) Influence of the size of the excitation region. For the data presented in the main text, we used an excitation size of 25%.

[†]Present address: Fakultät für Physik, Ludwig-Maximilians-Universität München, Schellingstr. 4, 80799 Munich, Germany.

[*] beugnon@lkb.ens.fr; [†]Present address: Fakultät für Physik, Ludwig-Maximilians-Universität München, Schellingstr. 4,

80799 Munich, Germany.

[1] K. Hueck, N. Luick, L. Sobirey, J. Siegl, T. Lompe, and H. Moritz, "Two-dimensional homogeneous fermi gases," Phys. Rev. Lett. **120**, 060402 (2018).

[2] A. Ramanathan, S.R. Muniz, K.C. Wright, R.P. Anderson, W.D. Phillips, K. Helmerson, and G.K. Campbell, "Partial-transfer absorption imaging: A versatile technique for optimal imaging of ultracold gases," Rev. Sci. Instrum. **83**, 083119 (2012).

[3] L. Corman, J. L. Ville, R. Saint-Jalm, M. Aidelsburger, T. Bienaimé, S. Nascimbène, J. Dalibard, and J. Beugnon, "Transmission of near-resonant light through a dense slab of cold atoms," Phys. Rev. A **96**, 053629 (2017).

[4] M.F. Riedel, P. Böhi, Y. Li, T.W. Hänsch, A. Sinatra, and P. Treutlein, "Atom-chip-based generation of entanglement for quantum metrology," Nature **464**, 1170 (2012).

[5] M.-C. Chung and A.B. Bhattacherjee, "Damping in 2D and 3D dilute Bose gases," New J. Phys. **11**, 123012 (2009).

[6] V. Pastukhov, "Damping of Bogoliubov excitations at finite temperatures," J. Phys. A: Math. Theor. **48**, 405002 (2015).

[7] P.C. Hohenberg and P.C. Martin, "Microscopic theory of superfluid helium," Ann. Phys. **34**, 291–359 (1965).
